# Supplementary material for: Banded Matrix Operators for Gaussian Markov Models in the Automatic Differentiation Era
Source: arXiv:1902.10078 source file (2019-02-26)
Supplement: Supplementary file 1 [file appendix_experiments.tex]

\section{Experiments}

\subsection{GMRF on Porto graph}

\begin{figure}[h]
    \centering
    \includegraphics[width=.8\textwidth]{figures/porto/porto_latent}
    \caption{Representation of the value of the sample corresponding to the logarithm of the rate used in the Poisson distribution to generate the counts.}
    \label{fig:porto_latent}
\end{figure}

\begin{figure}[h]
    \centering
    \includegraphics[width=.8\textwidth]{figures/porto/porto_data}
    \caption{Observed number of counts after sampling from the Poisson distribution at each node. We choose here a non-linear colormap to emphasis the variations for small values of the counts.}
    \label{fig:porto_counts}
\end{figure}

\begin{figure}[h]
    \centering
    \begin{subfigure}[b]{0.45\textwidth}
        \includegraphics[width=\textwidth]{figures/porto/porto_HMC_vs_f}
        \caption{Comparison of HMC vs reference values.\\}
        \label{fig:comp_inf_1}
    \end{subfigure}
    \qquad
    \begin{subfigure}[b]{0.45\textwidth}
        \includegraphics[width=\textwidth]{figures/porto/porto_VI_vs_f}
        \caption{Comparison of VI vs reference values.}
        \label{fig:comp_inf_2}
    \end{subfigure}
    \\ \ \\
    \begin{subfigure}[b]{0.45\textwidth}
        \includegraphics[width=\textwidth]{figures/porto/porto_HMC_vs_VI}
        \caption{Comparison mean predictions HMC vs VI.}
        \label{fig:comp_inf_3}
    \end{subfigure}
    \qquad
    \begin{subfigure}[b]{0.45\textwidth}
        \includegraphics[width=\textwidth]{figures/porto/porto_HMC_vs_VI_var}
        \caption{Comparaison variance prediction HMC vs VI.}
        \label{fig:comp_inf_4}
    \end{subfigure}
    \caption{Comparison of the models fitted on the Porto experiment.}
    \label{fig:porto_comp_inference}
\end{figure}
